# Supplementary material for: Unsupervised Traffic Scene Generation with Synthetic 3D Scene Graphs
Source: arXiv:2303.08473 source file (2023-03-15)
Supplement: Supplementary file 1 [file figure_sg_layout_sm_pfd_cs.tex]

\begin{figure*}[t!]
    \centering
    \includegraphics[width=0.95\textwidth]{images_tmp/graph_with_background.png}
    \includegraphics[width=0.95\textwidth]{images_tmp/graph_proc_setup_2.png}
    \caption{Layouts (bottom) produced from the corresponding synthetic scene graphs (top) along with ground-truth layouts(middle). Colors follow Cityscapes protocol.}
    \label{fig:layouts1}
\end{figure*}
